# Supplementary material for: Shrink-Perturb Improves Architecture Mixing during Population Based Training for Neural Architecture Search
Source: arXiv:2307.15621 source file (2023-07-28)

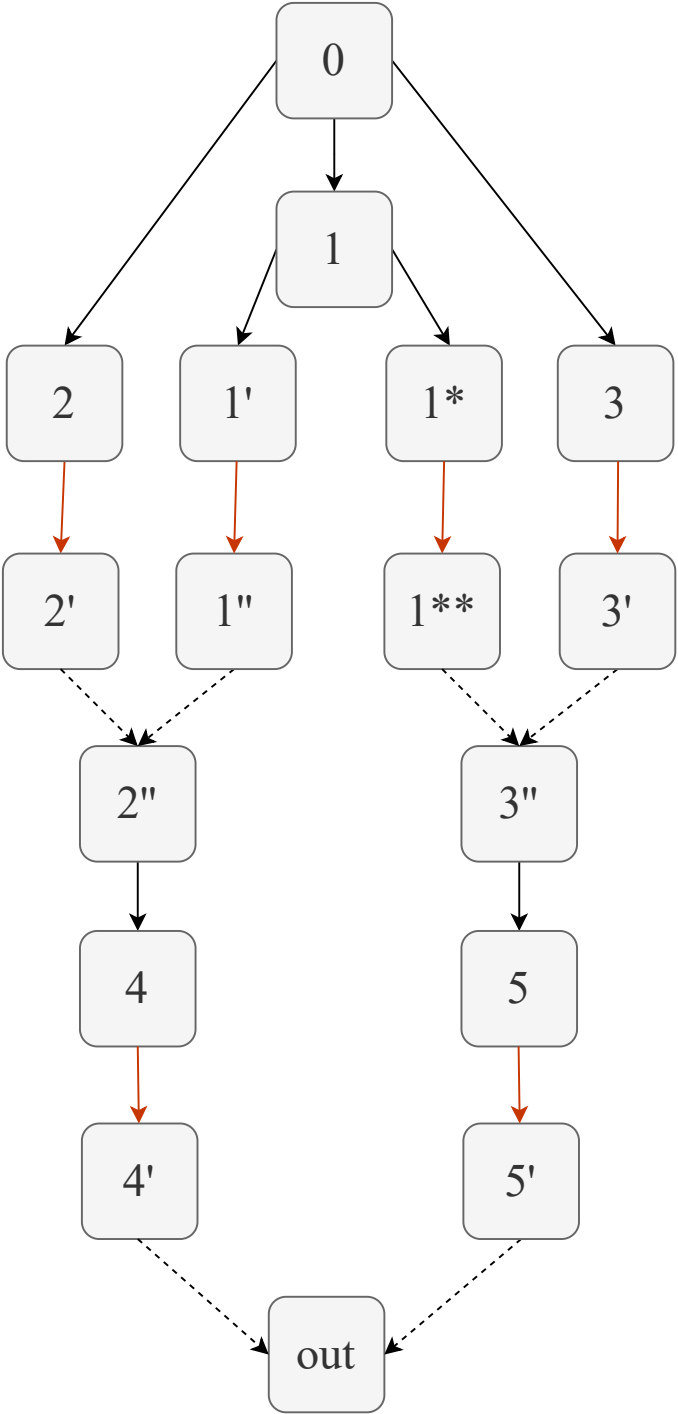

Supplement: Supplementary file 1 [file cell_my.pdf]
